# Supplementary material for: Correlating Gravitational Waves with $W$-boson Mass, FIMP Dark Matter, and Majorana Seesaw Mechanism
Source: arXiv:2204.04834 source file (2022-06-23)
Supplement: Supplementary file 1 [file Supplemental-File.pdf]

# Gravitational Wave Formulae

The GW spectrum today can be written as

$$\Omega_{\rm GW}(f) = \Omega_{\rm sw}(f) + \Omega_{\rm turb}(f), \tag{1}$$

where $\Omega_{\rm GW}$ is the ratio of GW energy density to the critical energy of the current Universe, i.e.,

$$\Omega_{\rm GW}(f) = \frac{1}{\rho_c}\frac{d\rho_{\rm GW}}{d\ln f}, \tag{2}$$

here $\rho_c = 3H_0^2/(8\pi G)$, with $H_0$ being the Hubble constant today. The sound wave and turbulence spectra can be expressed as functions of two important parameters [1, 2, 3],

$$\begin{aligned} \alpha &= \frac{1}{g_* \pi^2 T_n^4/30}\left(T\frac{\partial \Delta V_T}{\partial T} - \Delta V_T\right)\Big|_{T_n}, \\ \frac{\beta}{H} &= T_n \frac{d(S_3/T)}{dT}\Big|_{T_n}. \end{aligned} \tag{3}$$

The parameter $\alpha$ is the ratio of the FOPT latent heat to the radiation energy, and $\beta/H$ is the inverse ratio of FOPT duration to the Universe expansion time scale. In the above $\Delta V_T$ denotes the (negative) effective potential difference between the true vacuum and the false vacuum, and $g_*$ is the number of relativistic degrees of freedom during the FOPT.

With $\alpha$ and $\beta/H$, the sound waves spectrum can be numerical written as [4]

$$\Omega_{\rm sw}(f)h^2 = 2.65\times 10^{-6}\frac{1}{\beta/H}\left(\frac{\kappa_v \alpha}{1+\alpha}\right)^2\left(\frac{g_*}{100}\right)^{-1/3}\times v_b\left(\frac{f}{f_{\rm sw}}\right)^3\left(\frac{7}{4+3(f/f_{\rm sw})^2}\right)^{7/2}, \tag{4}$$

the peak frequency locates at

$$f_{\rm sw} = 1.9\times 10^{-2}\ {\rm mHz}\times\frac{\beta/H}{v_b}\left(\frac{T_n}{100\ {\rm GeV}}\right)\left(\frac{g_*}{100}\right)^{1/6}. \tag{5}$$

We also should take into account the finite duration of the sound wave period. To do that we make the replacement $\Omega_{\rm sw}(f) \to \Omega_{\rm sw}(f)H(T_n)\tau_{\rm sw}$ in Eq. 4 [5, 6], where

$$\begin{aligned} \tau_{\rm sw} &= \min\left\{\frac{1}{H(T_n)}, \frac{v_b(8\pi)^{1/3}}{\beta \bar{U}_f}\right\}, \\ \bar{U}_f &= \sqrt{\frac{3}{4}\frac{\kappa_v\alpha}{1+\alpha}}. \end{aligned} \tag{6}$$

A more accurate treatment for the sound wave cutoff factor can be found in Ref. [7].

For the turbulence source, the spectrum reads [8, 9]

$$\Omega_{\rm turb}(f)h^2 = 3.35\times 10^{-4}\frac{v_b}{\beta/H}\left(\frac{\kappa_{\rm turb}\alpha}{1+\alpha}\right)^{3/2}\times\left(\frac{g_*}{100}\right)^{-1/3} S_{\rm turb}(f), \tag{7}$$

with functions

$$S_{\rm turb}(f) = \frac{(f/f_{\rm turb})^3}{[1+(f/f_{\rm turb})]^{11/3}(1+8\pi f/h_*)}, \tag{8}$$

$$h_* = 16.5 \times 10^{-3}\ \mathrm{mHz} \left(\frac{T_n}{100\ \mathrm{GeV}}\right) \left(\frac{g_*}{100}\right)^{1/6} , \tag{9}$$

$$f_{\mathrm{turb}} = 2.7 \times 10^{-2}\ \mathrm{mHz} \times \frac{\beta/H}{v_b} \left(\frac{T_n}{100\ \mathrm{GeV}}\right) \left(\frac{g_*}{100}\right)^{1/6} . \tag{10}$$

In the above equations, $v_b$ is the bubble wall velocity, taken to be $v_b = 0.6$ in this work, $\kappa_v$ describes the fraction of latent heat transformed into the bulk motion of the fluid, which is extracted from the numerical function of Ref. [10]. We also have adopted $\kappa_{\mathrm{turb}} = 0.05\kappa_v$ in this study.

## REFERENCES


[1] C. Grojean and G. Servant, Phys. Rev. D **75**, 043507 (2007) doi:10.1103/PhysRevD.75.043507 [arXiv:hep-ph/0607107 [hep-ph]].

[2] C. Caprini, M. Hindmarsh, S. Huber, T. Konstandin, J. Kozaczuk, G. Nardini, J. M. No, A. Petiteau, P. Schwaller and G. Servant, *et al.* JCAP **04**, 001 (2016) doi:10.1088/1475-7516/2016/04/001 [arXiv:1512.06239 [astro-ph.CO]].

[3] C. Caprini, M. Chala, G. C. Dorsch, M. Hindmarsh, S. J. Huber, T. Konstandin, J. Kozaczuk, G. Nardini, J. M. No and K. Rummukainen, *et al.* JCAP **03**, 024 (2020) doi:10.1088/1475-7516/2020/03/024 [arXiv:1910.13125 [astro-ph.CO]].

[4] M. Hindmarsh, S. J. Huber, K. Rummukainen and D. J. Weir, Phys. Rev. D **92**, no.12, 123009 (2015) doi:10.1103/PhysRevD.92.123009 [arXiv:1504.03291 [astro-ph.CO]].

[5] J. Ellis, M. Lewicki and J. M. No, JCAP **07**, 050 (2020) doi:10.1088/1475-7516/2020/07/050 [arXiv:2003.07360 [hep-ph]].

[6] X. Wang, F. P. Huang and X. Zhang, JCAP **05**, 045 (2020) doi:10.1088/1475-7516/2020/05/045 [arXiv:2003.08892 [hep-ph]].

[7] H. K. Guo, K. Sinha, D. Vagie and G. White, JCAP **01**, 001 (2021) doi:10.1088/1475-7516/2021/01/001 [arXiv:2007.08537 [hep-ph]].

[8] P. Binetruy, A. Bohe, C. Caprini and J. F. Dufaux, JCAP **06**, 027 (2012) doi:10.1088/1475-7516/2012/06/027 [arXiv:1201.0983 [gr-qc]].

[9] C. Caprini, R. Durrer and G. Servant, JCAP **12**, 024 (2009) doi:10.1088/1475-7516/2009/12/024 [arXiv:0909.0622 [astro-ph.CO]].

[10] J. R. Espinosa, T. Konstandin, J. M. No and G. Servant, JCAP **06**, 028 (2010) doi:10.1088/1475-7516/2010/06/028 [arXiv:1004.4187 [hep-ph]].
